# Supplementary material for: AWorld: Orchestrating the Training Recipe for Agentic AI
Source: arXiv:2508.20404 source file (2025-09-01)
Supplement: Supplementary file 1 [file appendix.tex]

\section{Appendix A}
